# Supplementary material for: Capturing Turbulent Dynamics and Statistics in Experiments with Unstable Periodic Orbits
Source: arXiv:2008.02367 ancillary file (2020-08-04)
Supplement: Supplementary file 1 [file SupplementalMaterial.pdf]

# Supplemental Material

In this document we provide information supplementary to that discussed in the article "Capturing Turbulent Dynamics and Statistics in Experiments with Unstable Periodic Orbits"

## I. EXPERIMENTAL SETUP

The experimental setup employed in this study is very similar to those detailed in Refs. [11, 33, 36]. A quasi-two-dimensional flow is generated by driving a shallow electrolyte-dielectric bilayer using a horizontal, spatially (near) sinusoidal electromagnetic forcing. To create such a forcing, we arrange 14 NdFeB magnets (grade N42) to form an array of dimensions $15.24\,\mathrm{cm}\times(14\times 1.27\,\mathrm{cm})\times 0.32\,\mathrm{cm}$, as shown in Fig.1(a) of the main text. Adjacent magnets have opposite polarity, resulting in a nearly sinusoidal magnetic field $\mathbf{B} \approx B_0 e^{-\pi z/w}\sin(\pi y/w)\hat{\mathbf{z}}$ at the center of the array. Here, $w = 1.27\,\mathrm{cm}$ is the width of each magnet and $B_0 \approx 0.2$ T is the magnetic field strength at the surface of a magnet. The magnet array is placed on a horizontal aluminum plate and is padded with 0.32 cm thick aluminum bars to create a flat surface. A 50 $\mu$m-thick black contact paper is placed over this flat surface to provide uniform black background for better flow visualization. Acrylic bars and copper electrodes, running parallel to $y$ and $x$ axes respectively, are glued on top of contact paper to create a rectangular container of dimensions $17.8\,\mathrm{cm}\times 22.9\,\mathrm{cm}$ with the magnet array at its center. We note that the magnetic field is sinusoidal only near the center of the magnet array. Near the lateral boundaries of the container, it decays to zero as shown in Fig. 2 in Ref. [33].

To create a nearly horizontal flow, we use the two-immiscible-fluid-layer configuration shown in Fig. 1(b) of the main text. The bottom layer is a dielectric (perfluorooctane with density $\rho = 1769$ kg/m$^3$ and viscosity $\mu = 1.3$ mPa·s) and the top one is an electrolyte (1 M $CuSO_4$ with 40% glycerol by weight with density $\rho = 1160$ kg/m$^3$ and viscosity $\mu = 5.7$ mPa·s); each layer is $0.3\pm 0.003\,\mathrm{cm}$ thick. Passing a uniform direct current of density $\mathbf{J} = J\hat{\mathbf{y}}$ through the electrolyte generates a nearly sinusoidal Lorentz force $\mathbf{F} \approx B_0 J e^{-\pi z/w}\sin(\pi y/w)\,\hat{\mathbf{x}}$ that drives the electrolyte layer. Viscous coupling between the fluid layers also generates a horizontal flow in the bottom dielectric layer [32]. The solid boundary at the bottom of the fluid layers creates a vertical gradient in the horizontal velocity, rendering the flow Q2D. All of our experimental runs were carried out for current densities in the range $J \in [37.5, 41.5]$ A/m$^2$. Lastly, the temperature of the fluid layers is maintained constant (20±0.1C) by placing the aluminum container in a temperature-controlled water bath.

The flow in the experiment is visualized by seeding the electrolyte-dielectric interface with 25 micron Titanium dioxide ($TiO_2$) coated hollow glass spheres. Two arrays of LEDs running parallel to the acrylic side walls illuminate the tracer particles. Images of the entire horizontal extent of the flow are recorded at 15 Hz using a CCD camera with sensor resolution of 1024×768 pixels. Spatiotemporally resolved velocity fields at the electrolyte-dielectric interface $\mathbf{u}_i(x, y, t)$ are calculated using the Prana PIV package [30] employing the "Deform" multigrid PIV algorithm. The grid resolution of the resulting PIV measurements is $120 \times 160$, or approximately 9 grid points per magnet width. Due to the vertical gradient in the magnitude of horizontal velocity in a Q2D flow, the velocity fields at the electrolyte-air interface $\mathbf{u}(x, y, t)$ and electrolyte-dielectric interface $\mathbf{u}_i(x, y, t)$ are related by a scale factor $s = 1.08$, i.e., $\mathbf{u}(x, y, t) \approx s\mathbf{u}_i(x, y, t)$ [32, 33]. All comparison between experiment and direct numerical simulation (DNS) employed $\mathbf{u}(x, y, t)$ that corresponds to the electrolyte-air interface.

The dynamical regimes in the experiment (as well as the DNS) are parametrized using the

nondimensional Reynolds number, which we define as:

$$Re = \frac{U_{rms} w}{\nu}. \tag{S1}$$

Here, $\nu = 3.23 \times 10^{-6}$ m$^2$/s is the depth-averaged kinematic viscosity of the two fluid layers [32]. The characteristic velocity $U_{rms}$ is defined as the spatial root-mean-square average of $\mathbf{u}(x, y, t)$ over the central $8w \times 8w$ region of the flow domain which is subsequently temporally averaged over the entire time-series. Experimental results presented in this article correspond to $Re = 23.5 \pm 1.5$.

## II. 2D MODEL AND DNS

The 2D model in its dimensional form is:

$$\partial_t \mathbf{u} + \beta \mathbf{u} \cdot \nabla \mathbf{u} = -\frac{1}{\rho} \nabla p + \nu \nabla^2 \mathbf{u} - \alpha \mathbf{u} + \frac{1}{\rho} \langle \mathbf{F} \rangle_z, \tag{S2}$$

which was derived by depth-averaging the 3D Navier-Stokes equation along the confined direction $z$ [32]. Here, $\mathbf{u}(x, y, t)$ corresponds to the velocity field at the electrolyte-air interface in the experiment. The parameters $\nu$ and $\rho$ represent depth-averaged kinematic viscosity and density, respectively, $\alpha$ is the friction coefficient, and $\beta$ is the prefactor to the nonlinear term. Lastly, $\langle \mathbf{F} \rangle_z$ is the depth-averaged forcing density. For the experimental setup detailed above, $\beta = 0.80$, $\nu = 3.23 \times 10^{-6}$ m$^2$/s, $\alpha = 0.077$ s$^{-1}$, and $\rho = 959$ kg/m$^3$.

Choosing $U = U_{rms}$, $L = w$ (magnet width), $T = L/U = w/U_{rms}$, and $P = \rho U_{rms}^2$ as the velocity, length, time, and pressure scales, respectively, we nondimensionalize Eq. S2 to obtain the governing equation (1) in the main text:

$$\partial_t \mathbf{u} + \beta \mathbf{u} \cdot \nabla \mathbf{u} = -\nabla p + \frac{1}{Re} (\nabla^2 \mathbf{u} - \gamma \mathbf{u}) + \mathbf{f}, \tag{S3}$$

where $\gamma = \alpha w^2/\nu$ and $\mathbf{f} = w/\rho U_{rms}^2 \langle \mathbf{F} \rangle_z$ is the normalized forcing profile.

Direct numerical simulation (DNS) of the flow was performed using a second-order (in both space and time) discretization of the 2D model. The same numerical integrator was previously employed in Refs. [11, 19, 33, 36]. Velocity and pressure fields are spatially discretized on a 2D staggered grid of dimensions 280×360. This corresponds to a resolution of 20 cells per magnet width $w$, with grid spacing $\delta x/w = \delta y/w = 0.05$. Spatial derivatives in the 2D model are approximated using second-order central finite differences. Temporal integration of the 2D model is performed using a semi-implicit projection scheme to enforce incompressibility of the velocity field at each time step [33]. The temporal update of velocity employs second-order implicit Crank-Nicolson scheme for the linear terms and second-order explicit Adams-Bashforth scheme for the nonlinear term. For all numerical data presented in this article, a time step $\delta t = 1/110$ was used for temporal integration to ensure the CFL number $\max\{u_x, u_y\} \delta t/\delta x \leq 0.5$. Lastly, the depth-averaged forcing $\langle \mathbf{F} \rangle_z$ in the 2D model was computed using a dipole lattice model for the magnet array in the experiment, as detailed in Ref. [33].

## III. DIMENSIONALITY OF THE CHAOTIC SET

The Lyapunov spectrum of the chaotic set was estimated using the continuous Gram-Schmidt orthogonalization procedure detailed in Ref. [34, 35]. At each point $\mathbf{u}(t)$ on the turbulent trajectory, the evolution of an infinitesimal perturbation $u$ to the state vector $\mathbf{u}$ is governed by the equation:

$$\frac{\partial u}{\partial t} + \beta (u \cdot \nabla \mathbf{u} + \mathbf{u} \cdot \nabla u) = -\nabla \phi + \frac{1}{Re} \left( \nabla^2 u - \gamma u \right), \tag{S4}$$

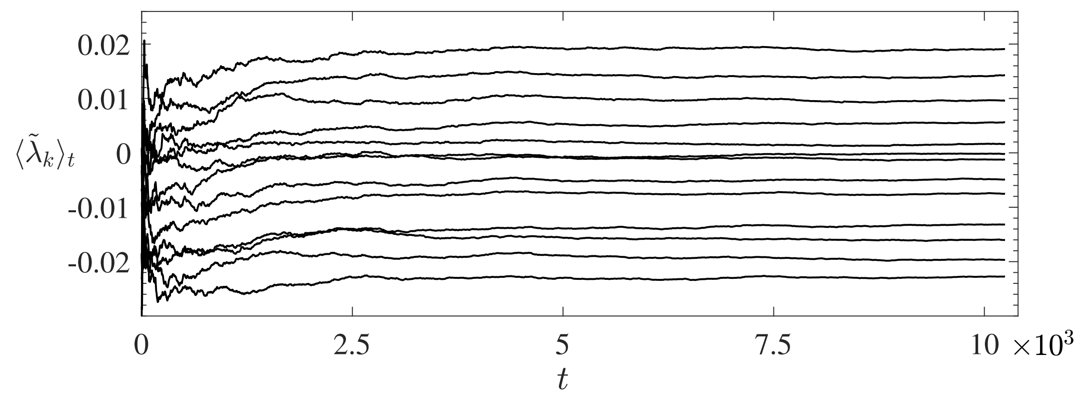


Fig. S1: Time-average of instantaneous Lyapunov spectra versus the duration of averaging. For very long trajectories ($t \gtrsim 10^4$), the average converges to the Lyapunov spectrum of the chaotic set. Only the first $k_0 + 1 = 13$ exponents are plotted.

which is obtained by linearizing Eq. S3 about $\mathbf{u}(t)$. The perturbation $u$ is divergence free ($\nabla \cdot u = 0$) and satisfies no-slip velocity boundary conditions. The amplitude of perturbation vector is chosen to be very small ($\eta = \|u\| = 10^{-4}$) in comparison to $\|\mathbf{u}\|(\approx O(100))$. Lastly, $\phi$ is the perturbation to pressure $p$ (cf. Eq. S3) and is computed using the Poisson equation obtained by taking the divergence of Eq. S4.

To compute the spectrum of Lyapunov exponents $\tilde{\lambda}_k$, we generate (at $t = 0$) a set of $N(= 40)$ mutually orthogonal random perturbation vectors $u_0^k$, i.e., $u_0^k \cdot u_0^j = \eta^2 \delta_{jk}$ (Kronecker delta) and $k, j = 1, 2, \cdots N$. For each $u_0^k$, Eq. S4 is evolved for a short duration $\Delta T$ ($\approx 0.1$ nondimensional time units); the turbulent trajectory is simultaneously evolved using Eq. S3. At $t = \Delta T$, the updated perturbation vectors $\tilde{u}_{\Delta T}^k$ are no longer mutually orthogonal. Using the modified Gram-Schmidt procedure, an orthogonal set of vectors $u_{\Delta T}^k$ is constructed from $\tilde{u}_{\Delta T}^k$ and the instantaneous Lyapunov spectrum is estimated using the relation:

$$\tilde{\lambda}_k = \frac{1}{\Delta T} \log \frac{\|u_{\Delta T}^k\|}{\|u_0^k\|} \tag{S5}$$

The perturbation vectors $u_{\Delta T}^k$ are finally rescaled to have an amplitude $\eta$ and used as initial conditions for the next iteration. When this procedure is carried out on a ($\approx 10^4$ nondimensional time units) long turbulent trajectory, the time average of $\tilde{\lambda}_k$ converges to the first $N$ Lyapunov exponents $\lambda_k$ of the chaotic set. Fig. S1 shows the convergence of the spectrum as the integration time is increased. The Kaplan-Yorke dimension of the chaotic set is computed from the Lyapunov spectrum as follows:

$$D_{KY} = k_0 + \frac{1}{|\lambda_{k_0+1}|} \sum_{k=1}^{k_0} \lambda_k, \tag{S6}$$

where the Lyapunov exponents $\lambda_k$ are sorted in descending order and $k_0$ is the largest integer for which the sum on the right-hand-side of Eq. S6 is non-negative.

## IV. PROPERTIES OF UNSTABLE PERIODIC ORBITS

The following properties of the seven UPOs are listed in Table SI:

- Period $T$ of the orbit in units of the Lyapunov time $\tau_l = 50\,\mathrm{s}$

| | $T/\tau_l$ | $N_u$ | $D_{KY}$ | $\lvert\Lambda_1\rvert$ | $\Pi_k\lvert\Lambda_k\rvert$ | $D_{po}/D_c$ | $\max\Delta\mathcal{R}$ | $\min\Delta\mathcal{R}$ |
|---|---|---|---|---|---|---|---|---|
| $\mathrm{UPO}_0$ | 0.67 | 5 | 12.47 | 7.95 | 10.97 | 0.17 | 0 | 0 |
| $\mathrm{UPO}_1$ | 0.70 | 3 | 11.09 | 2.53 | 12.5 | 0.15 | 0 | 0 |
| $\mathrm{UPO}_{2\mathrm{A}}$ | 1.31 | 4 | 8.06 | 27.4 | 76.6 | 0.64 | 0.32 | 0.29 |
| $\mathrm{UPO}_{2\mathrm{B}}$ | 1.36 | 1 | 2.32 | 1.32 | 1.32 | 0.58 | 0.29 | 0.26 |
| $\mathrm{UPO}_{2\mathrm{C}}$ | 1.42 | 2 | 4.43 | 1.99 | 3.16 | 0.55 | 0.28 | 0.25 |
| $\mathrm{UPO}_{3\mathrm{A},3\mathrm{B}}$ | 2.27 | 2 | 7.01 | 5.65 | 8.53 | 0.33 | 0.14 | 0.10 |

Table. SI: Properties of unstable periodic orbits

- Number $N_u$ of unstable directions
- Kaplan-Yorke dimension $D_{KY}$ of the linear neighborhood of each periodic orbit
- Magnitude of the leading Floquet multiplier, $|\Lambda_1|$
- Product of unstable Floquet multipliers, $\Pi_k|\Lambda_k| = |\Lambda_1||\Lambda_2|\cdots|\Lambda_k|$
- Diameter of the orbit $D_{po} = \max\limits_{0<t',t<T} \|\mathbf{u}_{po}(t) - \mathbf{u}_{po}(t')\|$ in units of the diameter $D_c = \max\limits_{t,t'} \|\mathbf{u}(t) - \mathbf{u}(t')\|$ of the chaotic set
- Maximum deviation of instantaneous flow field on a UPO from rotational symmetry, $\max\Delta\mathcal{R} = \max\limits_{t'} \|\mathbf{u}_{po}(t') - \mathcal{R}\mathbf{u}_{po}(t')\|/(2D_c)$
- Minimum deviation of instantaneous flow field on a UPO from rotational symmetry, $\min\Delta\mathcal{R} = \min\limits_{t'} \|\mathbf{u}_{po}(t') - \mathcal{R}\mathbf{u}_{po}(t')\|/(2D_c)$

## V. STATE SPACE PROJECTION

Fig. 2(a) in the main text is a low-dimensional projection of the high-dimensional state space, constructed to visualize the turbulent trajectory shadowing $\mathrm{UPO}_{3\mathrm{A}}$. For this projection, we followed a procedure similar to that described in Ref. [8]. To begin, we choose four flow snapshots:

$$\mathbf{u}_0 = \langle \mathbf{u}_{po}(t') \rangle_{t'}, \quad \mathbf{u}_1 = \mathbf{u}_{po}(t'_1), \quad \mathbf{u}_2 = \mathbf{u}_{po}(t'_2), \quad \mathbf{u}_3 = \langle \mathbf{u}(t) \rangle_t. \tag{S7}$$

Here, $\mathbf{u}_0$ is the time-averaged flow of the periodic orbit $\mathrm{UPO}_{3\mathrm{A}}$, $\mathbf{u}_1$ and $\mathbf{u}_2$ are two points on $\mathrm{UPO}_{3\mathrm{A}}$ that are sufficiently far apart from each other, and $\mathbf{u}_3$ is the mean turbulent flow, averaged over the interval the turbulent trajectory lies in the neighborhood of $\mathrm{UPO}_{3\mathrm{A}}$, i.e, $D_1(t) < 0.45$. We then construct three vectors:

$$\mathbf{v}_1 = \mathbf{u}_1 - \mathbf{u}_0 \quad \mathbf{v}_2 = \mathbf{u}_2 - \mathbf{u}_0 \quad \mathbf{v}_3 = \mathbf{u}_3 - \mathbf{u}_0 \tag{S8}$$

To visualize shadowing, the state space is projected onto the subspace spanned by $\mathbf{v}_1$, $\mathbf{v}_2$, and $\mathbf{v}_3$. Among these vectors, $\mathbf{v}_1$ and $\mathbf{v}_2$ represent the shape and orientation of $\mathrm{UPO}_{3\mathrm{A}}$, while $\mathbf{v}_3$ captures the average deviation of the turbulent trajectory from $\mathrm{UPO}_{3\mathrm{A}}$. The vectors $\mathbf{v}_1, \mathbf{v}_2$, and $\mathbf{v}_3$ are typically not mutually orthogonal. Hence, we construct an orthonormal set of vectors $\hat{\mathbf{e}}_1$, $\hat{\mathbf{e}}_2$, $\hat{\mathbf{e}}_3$

from $\mathbf{v}_1, \mathbf{v}_2, \mathbf{v}_3$ using Gram-Schmidt orthonormalization. The projections of state space trajectories onto $\hat{\mathbf{e}}_1$, $\hat{\mathbf{e}}_2$, $\hat{\mathbf{e}}_3$ are given by the scalar products:

$$c_i(t) = \hat{\mathbf{e}}_i \cdot (\mathbf{u}(t) - \mathbf{u}_0), \tag{S9}$$

where $\mathbf{u}(t)$ corresponds to either the turbulent trajectory or $\mathbf{u}_{po}(t)$. We note that the procedure described here was also employed in Fig. S1 and S2, which show turbulent trajectories in experiment shadowing UPO$_0$ and UPO$_{2B}$. In each case, the basis vectors are constructed from the UPO being shadowed and the segment of turbulent trajectory in its vicinity.

## VI. TURBULENT TRAJECTORIES SHADOWING UPO$_0$ AND UPO$_{2B}$

In the main text we showed that turbulent trajectories in experiment approach UPO$_{3A}$ and shadow its evolution (cf. Figs. 2 and 3). Using a similar analysis, we also identified that solutions UPO$_0$ and UPO$_{2B}$ are shadowed by the turbulent flow in experiment for extended periods of time. A pair of such events is described here.

Fig. S2(a) shows a segment of turbulent trajectory $\mathbf{u}(t)$ in experiment shadowing UPO$_0$ for a duration that is approximately equal to one period of UPO$_0$ ($T = 0.67\tau_l$). Over this interval, the distance between $\mathbf{u}(t)$ and UPO$_0$ is below $D_1 = 0.45$ and instantaneous snapshots from the turbulent flow and its UPO counterpart, indicated by symbols in Fig. S2(a), are strikingly similar. As Fig. S2(d) shows, the turbulent flow evolves at a slightly slower rate compared to UPO$_0$. Video 2 shows side-by-side comparison of turbulent flow and UPO$_0$ in both state space and physical space.

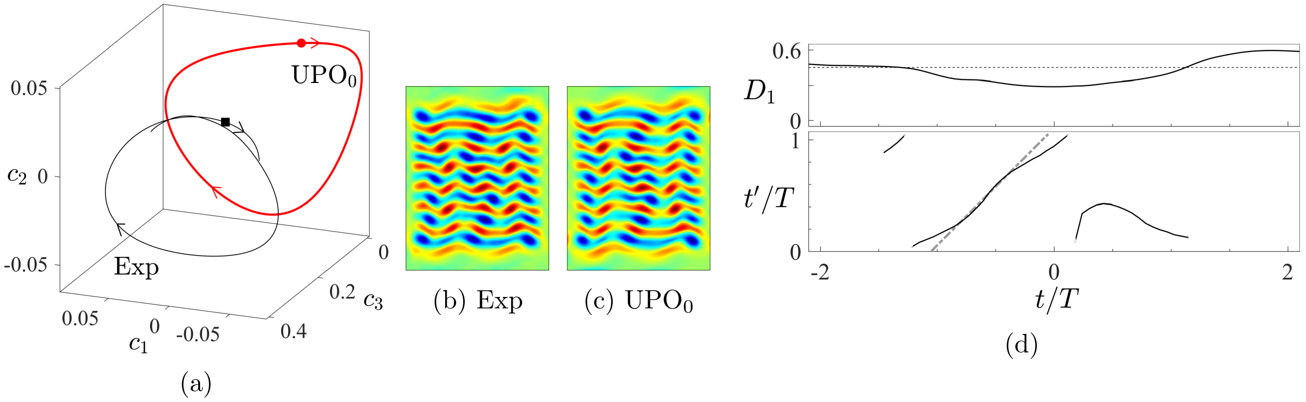


Fig. S2: Turbulent trajectory $\mathbf{u}(t)$ from experiment shadowing UPO$_0$ (a) Low-dimensional projection of state space showing UPO$_0$ (red curve) and $\mathbf{u}(t)$ (black curve). Sphere and square mark points on UPO$_0$ and the turbulent trajectory which are instantaneously the closest. (b,c) The corresponding flow snapshots; here, color represents vorticity $\omega = (\nabla \times \mathbf{u}) \cdot \hat{\mathbf{z}}$. (d) Instantaneous separation $D_1$ between $\mathbf{u}(t)$ and UPO$_0$ as well as the corresponding times $t$ and $t'$ that parametrize position along $\mathbf{u}(t)$ and UPO$_0$, respectively.

Fig. S3(a) shows a segment of turbulent trajectory from experiment shadowing UPO$_{2B}$. Recall that UPO$_{2B}$ is a pre-periodic orbit, i.e., $\mathbf{u}_{po}(t' + T) = \mathcal{R}\mathbf{u}(t')$, where $T = 1.36\,\tau_l$. Consequently, the flow repeats exactly after every two periods, as shown in Fig. S3 (red loop). Here, the segments plotted using solid and dashed curves are each one period long. UPO$_{2B}$ is shadowed by the turbulent trajectory for a duration slightly longer than three periods: as Fig. S3(d) illustrates, the instantaneous separation $D_1(t)$ between $\mathbf{u}(t)$ and UPO$_{2B}$ remains relatively small and the evolution rates ($t'$ vs $t$) remain comparable. Video 3 shows side-by-side comparison of turbulent flow and UPO$_{2B}$ in both state space and physical space.

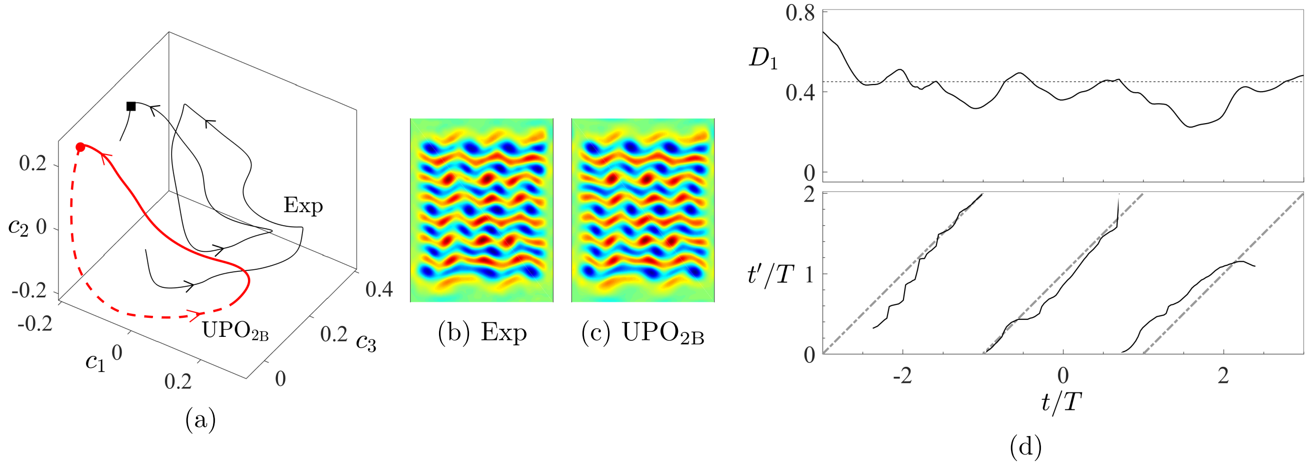


Fig. S3: Turbulent trajectory $\mathbf{u}(t)$ from experiment shadowing UPO$_{2B}$ (a) Low-dimensional projection of state space showing two-periods of UPO$_{2B}$ and $\mathbf{u}(t)$ (black curve). The solid and dashed red curves indicate one-period long segments along UPO$_{2B}$. The sphere and square mark points on UPO$_{2B}$ and $\mathbf{u}(t)$, respectively, which are instantaneously the closest. (b,c) The corresponding flow snapshots (d) Instantaneous separation $D_1$ between $\mathbf{u}(t)$ and UPO$_{2B}$ as well as the times $t$ and $t'$ that parametrize position along $\mathbf{u}(t)$ and UPO$_{2B}$, respectively.

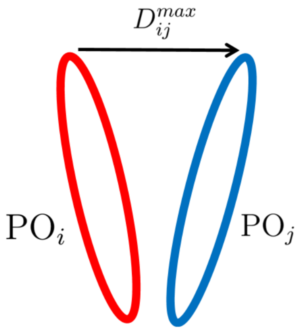


Fig. S4: A cartoon illustrating the geometrical interpretation of $D_{ij}^{max}$.

## VII. CLUSTERING OF UPOs

To distinguish the statistical significance of various UPOs, we clustered UPOs which are adjacent to each other in state space. A turbulent flow is often simultaneously close to all UPOs within a cluster. To identify nearby UPOs, we computed the quantity

$$D_{ij}^{max} = D_c^{-1} \max_t \min_{t'} \|\mathbf{u}_{po}^i(t) - \mathbf{u}_{po}^j(t')\|. \tag{S10}$$

which defines the maximum distance from UPO$_i$ to the closest point on UPO$_j$. The geometrical interpretation of $D_{ij}^{max}$ is illustrated schematically in Fig. S4. Two UPOs in state space can be regarded as adjacent to each other if $D_{ij}^{max} < 0.45$. Table 2 lists $D_{ij}^{max}$ for the various UPO pairs. Clearly, our analysis reveals three UPO clusters, UPO$_{0,1}$, UPO$_{2A\text{-}2C}$, and UPO$_{3A,3B}$, which are highlighted using different colors in the Table.

Table 2: Distance $D_{ij}^{max}$ between UPO pairs.

| | $UPO_0$ | $UPO_1$ | $UPO_{2A}$ | $UPO_{2B}$ | $UPO_{2C}$ | $UPO_{3A}$ | $UPO_{3B}$ |
|---|---|---|---|---|---|---|---|
| $UPO_0$ | - | 0.20 | 0.55 | 0.57 | 0.57 | 0.67 | 0.67 |
| $UPO_1$ | 0.20 | - | 0.54 | 0.54 | 0.54 | 0.67 | 0.67 |
| $UPO_{2A}$ | 0.57 | 0.57 | - | 0.20 | 0.24 | 0.51 | 0.51 |
| $UPO_{2B}$ | 0.60 | 0.60 | 0.20 | - | 0.09 | 0.46 | 0.46 |
| $UPO_{2C}$ | 0.62 | 0.62 | 0.24 | 0.09 | - | 0.44 | 0.44 |
| $UPO_{3A}$ | 0.69 | 0.70 | 0.48 | 0.44 | 0.41 | - | 0.27 |
| $UPO_{3B}$ | 0.69 | 0.70 | 0.48 | 0.44 | 0.41 | 0.27 | - |

## VIII. COMPARISON OF WEIGHTING PROTOCOLS

In Fig. 4(b) of the main text we rationalized the relative statistical significance of the three UPO clusters using weights prescribed by POT Eq. (4). Two alternative weighting protocols have also been suggested previously by Zoldi *et al.* [39, 40]

$$\pi_i = \frac{1}{\sum \lambda_{ik}} \tag{S11}$$

and Kazantsev [37]

$$\pi_i = \frac{T_i}{\sum \lambda_{ik}}. \tag{S12}$$

In both expressions, the summation is over all unstable Floquet exponents $\lambda_{ik}$ of $UPO_i$, and $T_i$ is its period. As discussed in the main text, we defined the weight associated with each UPO cluster as $w_c \propto \sum \pi_i$, where the summation is over all UPOs in that cluster. Fig. S5 shows the weights associated with each cluster computed using the three protocols, as well as the weights ($w_c = P_c/P$) estimated using DNS. The three protocols yield qualitatively similar results. Previously, Chandler *et al.* [17] have reported that statistical averages computed as weighted sums over a fairly large (over 50) set of UPOs are similar for these three weighting protocols. On the other hand, Zoldi [40] argued that, for nonhyperbolic systems, the weighting protocol (S11) yields more accurate results than POT trace formulas for a set of over 500 orbits.

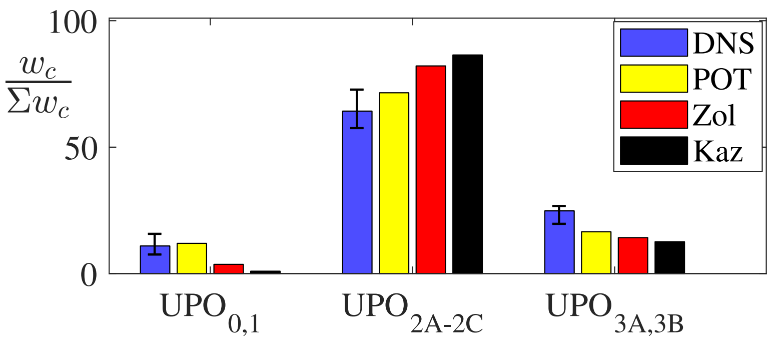


Fig. S5: Normalized weights associated with UPO clusters computed using DNS, POT (Eq. 4), and protocols of Zoldi (S11) and Kazantsev (S12).
